# Supplementary material for: POINTER: Constrained Progressive Text Generation via Insertion-based Generative Pre-training
Source: arXiv:2005.00558 source file (2020-09-27)
Supplement: Supplementary file 1 [file supp.pdf]

## Appendix

### A Baseline and Experimental Details

For NMSTG, we first convert the lexical constraints into a prefix sub-tree, and then sample a sentence to complete the sub-tree. We use the default settings suggested by the authors, and use an LSTM with hidden size of 1024 as the text generator, and select the best performed variants (*annealed*) as our baseline. For CGMH, we use their default setting, which uses an LSTM with hidden size of 300, and set the vocabulary size as 50k. Both models are trained until the evaluation loss does not decrease. During inference, we run CGMH for 500 iterations with default hyperparameters.

For experiment setup, we employ the tokenizer from BERT, and use WordPiece Embeddings (Wu et al., 2016) with a 30k token vocabulary for all the tasks. A special no-insertion token [NOI] is added to the vocabulary. We utilize the BERT-base and BERT-large models with 12 self-attention layers and 768 hidden dimension as our model initialization. Each model is trained until there is no progress on the validation loss. We use a learning rate of  $3e-5$  without any warming-up schedule for all the training procedures. The optimization algorithm is Adam (Kingma and Ba, 2015). We pre-train our model on the Wiki dataset for 2 epochs, and fine-tune on the News and Yelp datasets for around 10 epochs.

### B Additional Generated Examples for News Dataset

We provide two examples on News dataset for how the model progressively generates the sentences in Table 7. All the generations are from the POINTER large model using greedy decoding.

In this section, we also provide some additional examples from the 1k news test data.

| Stage       | Generated text sequence                                                                                                                                                                                                                           |
|-------------|---------------------------------------------------------------------------------------------------------------------------------------------------------------------------------------------------------------------------------------------------|
| 0 ( $X^0$ ) | aware negative immediately sites                                                                                                                                                                                                                  |
| 1 ( $X^1$ ) | if aware <b>posts</b> negative <b>should</b> immediately <b>any</b> sites <b>posts</b>                                                                                                                                                            |
| 2 ( $X^2$ ) | <b>would</b> if <b>user</b> aware <b>that</b> posts <b>have</b> negative <b>impact</b> should immediately <b>related</b> any <b>these</b> sites <b>remove</b> posts                                                                               |
| 3 ( $X^3$ ) | <b>this</b> would <b>prefer</b> if <b>the</b> user <b>is</b> aware that <b>the</b> posts have <b>a</b> negative impact <b>and</b> should <b>be</b> immediately related <b>to</b> any <b>of</b> these sites <b>and</b> remove <b>those</b> posts . |
| Stage       | Generated text sequence                                                                                                                                                                                                                           |
| 0 ( $X^0$ ) | estate pay stay policy                                                                                                                                                                                                                            |
| 1 ( $X^1$ ) | <b>also</b> estate <b>agents</b> pay <b>amount</b> stay <b>same</b> policy assets                                                                                                                                                                 |
| 2 ( $X^2$ ) | <b>it</b> also <b>required</b> estate agents <b>who</b> pay <b>same</b> amount <b>cash</b> stay <b>with</b> same policy <b>all</b> assets                                                                                                         |
| 3 ( $X^3$ ) | <b>but</b> it <b>would</b> also <b>be</b> required <b>for</b> estate agents , who <b>must</b> pay <b>the</b> same amount <b>of</b> cash <b>but</b> stay with <b>the</b> same policy <b>for</b> all <b>other</b> assets .                          |

Table 7: Example of the progressive generation process with multiple stages from the POINTER model. New additions at each stage are marked as **blue**.

| Keywords                | aware negative immediately sites                                                                                                                                                                                                  |
|-------------------------|-----------------------------------------------------------------------------------------------------------------------------------------------------------------------------------------------------------------------------------|
| ORACLE                  | where we become <b>aware</b> of any accounts that may be <b>negative</b> , we <b>immediately</b> contact companies such as Instagram , although we have no control over what they allow on their <b>sites</b> .                   |
| CGMH                    | not even <b>aware</b> of <b>negative</b> events including video events <b>immediately</b> at stations , Facebook <b>sites</b> .                                                                                                   |
| NMSTG                   | health providers in a country for England are <b>aware</b> of small health systems - and not non - health care but all <b>negative</b> is <b>immediately</b> treated by heads of businesses and departments in the <b>sites</b> . |
| POINTER (Greedy, base)  | ' if users are <b>aware</b> of the <b>negative</b> impact of blocking , how can they so <b>immediately</b> ban these <b>sites</b> ? ' the researchers wrote .                                                                     |
| POINTER (ILBS, base)    | if the users are <b>aware</b> of or the <b>negative</b> messages , they can <b>immediately</b> be transferred to other <b>sites</b> .                                                                                             |
| POINTER (Greedy, Large) | this would prefer if the user is <b>aware</b> that the posts have a <b>negative</b> impact and should be <b>immediately</b> related to any of these <b>sites</b> and remove those posts .                                         |
| Wiki zero-shot          | he is not <b>aware</b> of the <b>negative</b> , and will <b>immediately</b> go to the positive <b>sites</b> .                                                                                                                     |

|                         |                                                                                                                                                                                                                                |
|-------------------------|--------------------------------------------------------------------------------------------------------------------------------------------------------------------------------------------------------------------------------|
| Keywords                | children fault left charge                                                                                                                                                                                                     |
| ORACLE                  | my relationship with my <b>children</b> was seriously affected as they were told time and again that everything was my <b>fault</b> , they were even <b>left</b> ' in <b>charge</b> ' of me if my wife went out of the house . |
| CGMH                    | his two <b>children</b> are the rare <b>fault</b> that <b>left</b> the police <b>charge</b>                                                                                                                                    |
| NMSTG                   | but despite <b>children</b> from hospitals to last one by <b>fault</b> backing this month , there have arrived as Mr Hunt has been <b>left charge</b> .                                                                        |
| POINTER (Greedy, base)  | but i found that these <b>children</b> were not at school however this was not their <b>fault</b> , and if so they were <b>left</b> without a parent in <b>charge</b> .                                                        |
| POINTER (ILBS, base)    | but my lovely wife and <b>children</b> consider that it is not our own <b>fault</b> and we should not be <b>left</b> alone in <b>charge</b> .                                                                                  |
| POINTER (Greedy, Large) | i said to my <b>children</b> : it ' s not his <b>fault</b> the parents <b>left</b> him ; the parents should be in <b>charge</b> of him .                                                                                       |
| Wiki zero-shot          | but for the <b>children</b> who are not at a <b>fault</b> , they are <b>left</b> behind on the <b>charge</b> .                                                                                                                 |

|                         |                                                                                                                                                                         |
|-------------------------|-------------------------------------------------------------------------------------------------------------------------------------------------------------------------|
| Keywords                | estate pay stay policy                                                                                                                                                  |
| ORACLE                  | how many people on the <b>estate</b> does he think will be affected by the new <b>pay</b> - to - <b>stay policy</b> ?                                                   |
| CGMH                    | an economic <b>estate</b> developer that could <b>pay</b> for it is that a <b>stay policy</b>                                                                           |
| NMSTG                   | as <b>estate</b> owners , they cannot <b>pay</b> for households for hundreds of middle - income property , buyers <b>stay</b> in retail <b>policy</b> .                 |
| POINTER (Greedy, base)  | if you buy new buildings from real <b>estate</b> company, you may have to <b>pay</b> down a mortgage and <b>stay</b> with the <b>policy</b> for financial reasons .     |
| POINTER (ILBS, base)    | but no matter what foreign buyers do , real <b>estate</b> agents will have to <b>pay</b> a small fee to <b>stay</b> consistent with the <b>policy</b> .                 |
| POINTER (Greedy, Large) | but it would also be required for <b>estate</b> agents , who must <b>pay</b> a larger amount of cash but <b>stay</b> with the same <b>policy</b> for all other assets . |
| Wiki zero-shot          | however , his real <b>estate</b> agent agreed to <b>pay</b> him for the <b>stay</b> under the same <b>policy</b> .                                                      |

|                         |                                                                                                                                                                                           |
|-------------------------|-------------------------------------------------------------------------------------------------------------------------------------------------------------------------------------------|
| Keywords                | managers cut costs million                                                                                                                                                                |
| ORACLE                  | he was the third of four <b>managers</b> sent in to <b>cut costs</b> and deal with the city ' s \$ 13 <b>million</b> deficit .                                                            |
| CGMH                    | the <b>managers</b> , who tried to <b>cut</b> off their <b>costs</b> , added 20 <b>million</b> euros                                                                                      |
| NMSTG                   | business <b>managers cut</b> demand for more expensive <b>costs</b> in 2017 - by October - is around 5 <b>million</b> 8 per cent , and has fallen by 0 . 3 per cent in January and 2017 . |
| POINTER (Greedy, base)  | under one of its general <b>managers</b> , the firm had already <b>cut</b> its annual operating <b>costs</b> from \$ 13 . 5 <b>million</b> to six million euros .                         |
| POINTER (ILBS, base)    | and last month , the <b>managers</b> announced that it had <b>cut</b> its operating <b>costs</b> by \$ 30 <b>million</b> .                                                                |
| POINTER (Greedy, Large) | the biggest expense is for the <b>managers</b> , where it plans to <b>cut</b> their annual management <b>costs</b> from \$ 18 . 5 <b>million</b> to \$ 12 million .                       |
| Wiki zero-shot          | but then he and all of his <b>managers</b> agreed to <b>cut</b> off all of the operating <b>costs</b> by about 1 <b>million</b> .                                                         |

|                         |                                                                                                                                                                                       |
|-------------------------|---------------------------------------------------------------------------------------------------------------------------------------------------------------------------------------|
| Keywords                | looked report realized wife                                                                                                                                                           |
| ORACLE                  | i <b>looked</b> at the <b>report</b> and saw her name , and that's when I <b>realized</b> it was my ex- <b>wife</b> .                                                                 |
| CGMH                    | he <b>looked</b> at the <b>report</b> and said he <b>realized</b> that if his <b>wife</b> Jane                                                                                        |
| NMSTG                   | i <b>looked</b> at my <b>report</b> about before I <b>realized</b> I return to travel holidays but - it doesn ' t haven ' t made anything like my <b>wife</b> .                       |
| POINTER (Greedy, base)  | when i turned and <b>looked</b> at a file <b>report</b> from the airport and <b>realized</b> it was not my <b>wife</b> and daughter .                                                 |
| POINTER (ILBS, base)    | when i turned around and <b>looked</b> down at the pictures from the <b>report</b> , i <b>realized</b> that it was my <b>wife</b> .                                                   |
| POINTER (Greedy, Large) | however , when they <b>looked</b> at the details of the <b>report</b> about this murder , they quickly <b>realized</b> that the suspect was not with his <b>wife</b> or his partner . |
| Wiki zero-shot          | but when he <b>looked</b> up at the <b>report</b> , he <b>realized</b> that it was not his <b>wife</b> .                                                                              |

|                         |                                                                                                                                                                                           |
|-------------------------|-------------------------------------------------------------------------------------------------------------------------------------------------------------------------------------------|
| Keywords                | time claim tax year                                                                                                                                                                       |
| ORACLE                  | walker says there is still <b>time</b> to <b>claim</b> this higher protection if you haven ' t already as the deadline is the end of the 2016 / 2017 <b>tax year</b> .                    |
| CGMH                    | ” two states , one - <b>time</b> voters can <b>claim</b> a federal <b>tax year</b>                                                                                                        |
| NMSTG                   | this <b>time</b> they had three to <b>claim</b> of an equal <b>tax</b> and 34 women at which indicated they should leave that over the <b>year</b> of 16 .                                |
| POINTER (Greedy, base)  | it is the very first <b>time</b> in history that trump will ever <b>claim</b> over \$ 400 million in federal income <b>tax</b> that he had held last <b>year</b> , the same report says . |
| POINTER (ILBS, base)    | is this the very first <b>time</b> someone has to <b>claim</b> federal income <b>tax</b> twice in a single <b>year</b> ?                                                                  |
| POINTER (Greedy, Large) | this is not for the first <b>time</b> that the scottish government was able to <b>claim tax</b> cuts of thousands of pounds a <b>year</b> to pay .                                        |
| Wiki zero-shot          | but at the <b>time</b> , the <b>claim</b> was that the same sales <b>tax</b> that was from the previous fiscal <b>year</b> .                                                              |

|                         |                                                                                                                                                                 |
|-------------------------|-----------------------------------------------------------------------------------------------------------------------------------------------------------------|
| Keywords                | model years big drama                                                                                                                                           |
| ORACLE                  | the former <b>model</b> said : “ I haven ' t seen him in so many <b>years</b> , I can ' t make a <b>big drama</b> out of it . ”                                 |
| CGMH                    | the “ <b>model</b> ” continues , like many <b>years</b> of sexual and <b>big drama</b> going                                                                    |
| NMSTG                   | after <b>model</b> two <b>years</b> and did it like , could we already get bigger than others in a <b>big drama</b> ?                                           |
| POINTER (Greedy, base)  | but i am a good role <b>model</b> , who has been around for 10 <b>years</b> now , and that is a <b>big</b> example of what i can do in <b>drama</b> on screen . |
| POINTER (ILBS, base)    | but the young actress and <b>model</b> , for 15 <b>years</b> , made a very <b>big</b> impact on the <b>drama</b> .                                              |
| POINTER (Greedy, Large) | i have seen the different <b>model</b> she recommends of over <b>years</b> , but it ' s no <b>big</b> change in the <b>drama</b> after all .                    |
| Wiki zero-shot          | she was a <b>model</b> actress for many <b>years</b> and was a <b>big</b> star in the <b>drama</b> .                                                            |

|                         |                                                                                                                                                                                                   |
|-------------------------|---------------------------------------------------------------------------------------------------------------------------------------------------------------------------------------------------|
| Keywords                | made year resolution managed                                                                                                                                                                      |
| ORACLE                  | i once <b>made</b> this my new <b>year</b> ' s <b>resolution</b> , and it is the only one that I ' ve actually ever <b>managed</b> to keep .                                                      |
| CGMH                    | indeed , as he <b>made</b> up the previous <b>year</b> , the GOP <b>resolution</b> was <b>managed</b>                                                                                             |
| NMSTG                   | while additional sanctions had been issued last week <b>made</b> a <b>year</b> from the latest <b>resolution</b> , Russia ' s Russian ministers have but have <b>managed</b> .                    |
| POINTER (Greedy, base)  | no progress has been <b>made</b> in syria since the security council started a <b>year</b> ago , when a <b>resolution</b> expressed confidence that moscow <b>managed</b> to save aleppo .        |
| POINTER (ILBS, base)    | and the enormous progress we have <b>made</b> over the last <b>year</b> is to bring about a <b>resolution</b> that has not been <b>managed</b> .                                                  |
| POINTER (Greedy, Large) | the obama administration , which <b>made</b> a similar call earlier this <b>year</b> and has also voted against a <b>resolution</b> to crack down on the funding , <b>managed</b> to recover it . |
| Wiki zero-shot          | but despite all the same changes <b>made</b> both in both the previous fiscal <b>year</b> , and by the un <b>resolution</b> itself , only the federal government <b>managed</b> ...               |

|                         |                                                                                                                                                                                                             |
|-------------------------|-------------------------------------------------------------------------------------------------------------------------------------------------------------------------------------------------------------|
| Keywords                | club believed centre window                                                                                                                                                                                 |
| ORACLE                  | the <b>club</b> are <b>believed</b> to be keen on bringing in cover at <b>centre</b> - back during the current transfer <b>window</b> , with a loan move most likely .                                      |
| CGMH                    | the <b>club</b> has also been <b>believed</b> that more than a new <b>centre</b> - up <b>window</b>                                                                                                         |
| NMSTG                   | one <b>club believed</b> it was not clear that the <b>centre</b> would hold place on the <b>window</b> until there were no cases that they had heard or had the decision disappeared .                      |
| POINTER (Greedy, base)  | he had been talking to the <b>club</b> since he is <b>believed</b> to have reached the <b>centre</b> spot in the queue before the january transfer <b>window</b> was suspended .                            |
| POINTER (ILBS, base)    | when he left his old <b>club</b> , chelsea , he was <b>believed</b> to be at the <b>centre</b> of the transfer <b>window</b> .                                                                              |
| POINTER (Greedy, Large) | the striker has remained at the <b>club</b> at the weekend and is increasingly <b>believed</b> to be available as a <b>centre</b> of the club during the summer transfer <b>window</b> until january 2016 . |
| Wiki zero-shot          | during his first <b>club</b> as manager he was widely <b>believed</b> to be at the <b>centre</b> forward in the january transfer <b>window</b> .                                                            |

|                         |                                                                                                                                                     |
|-------------------------|-----------------------------------------------------------------------------------------------------------------------------------------------------|
| Keywords                | great past decade city                                                                                                                              |
| ORACLE                  | it ' s been a <b>great</b> time , the <b>past decade</b> or so , to be the mayor of a major capital <b>city</b> .                                   |
| CGMH                    | the great past decade is that so much of a new home city                                                                                            |
| NMSTG                   | i like to thank you for me and I ' ve wanted it to grow in every <b>great past decade</b> over the <b>city</b> , a very amazing time .              |
| POINTER (Greedy, base)  | this is one of the <b>great</b> cities that he have visited in the <b>past</b> two <b>decade</b> , the kansas <b>city</b> , missouri , he says .    |
| POINTER (ILBS, base)    | you don ' t feel as <b>great</b> as you ' ve been in the <b>past decade</b> in a major <b>city</b> .                                                |
| POINTER (Greedy, Large) | there has been a lot of <b>great</b> work here in the <b>past</b> few years within more than a <b>decade</b> , done for the <b>city</b> , he says . |
| Wiki zero-shot          | there was a <b>great</b> success in the <b>past</b> during the last <b>decade</b> for the <b>city</b> .                                             |

## C Additional Generated Examples for Yelp Dataset

We provide two examples on Yelp dataset for how the model progressively generates the sentences in Table 8. All the generations are from the POINTER large model using greedy decoding.

We also provide some additional examples from the Yelp test set. The results includes keywords, human oracle, CGMH, NMSTG and our models. For our models, we include POINTER base and large models with greedy decoding and base model with ILBS. The large model with ILBS is time consuming so we omit them from the comparison.

| Stage       | Generated text sequence                                                                                                                                                                                                                                                                                                                                                                                                                                                |
|-------------|------------------------------------------------------------------------------------------------------------------------------------------------------------------------------------------------------------------------------------------------------------------------------------------------------------------------------------------------------------------------------------------------------------------------------------------------------------------------|
| 0 ( $X^0$ ) | delicious love mole rice back                                                                                                                                                                                                                                                                                                                                                                                                                                          |
| 1 ( $X^1$ ) | <b>restaurant</b> delicious <b>authentic</b> love <b>dish</b> mole <b>beans</b> rice <b>definitely</b> back !                                                                                                                                                                                                                                                                                                                                                          |
| 2 ( $X^2$ ) | <b>new</b> restaurant <b>so</b> delicious <b>fresh</b> authentic . love <b>mexican</b> dish <b>called</b> mole <b>with</b> beans <b>and</b> rice <b>we</b> definitely <b>coming</b> back <b>more</b> !                                                                                                                                                                                                                                                                 |
| 3 ( $X^3$ ) | <b>this</b> new restaurant <b>is</b> so delicious , fresh <b>and</b> authentic <b>tasting</b> . <b>i</b> love <b>the</b> mexican <b>style</b> dish , called <b>the</b> mole , with <b>black</b> beans , and <b>white</b> rice . we <b>will</b> definitely <b>be</b> coming back <b>for</b> more !                                                                                                                                                                      |
| Stage       | Generated text sequence                                                                                                                                                                                                                                                                                                                                                                                                                                                |
| 0 ( $X^0$ ) | joint great food great drinks greater staff                                                                                                                                                                                                                                                                                                                                                                                                                            |
| 1 ( $X^1$ ) | <b>new</b> joint <b>around</b> great <b>location</b> food <b>variety</b> great <b>craft</b> drinks <b>unless</b> greater <b>friendly</b> staff !                                                                                                                                                                                                                                                                                                                       |
| 2 ( $X^2$ ) | <b>is</b> new <b>breakfast</b> joint <b>be</b> around <b>area</b> great , location <b>excellent</b> food <b>nice</b> variety <b>selections</b> great <b>of</b> craft , drinks <b>quite</b> unless <b>ask</b> greater . friendly <b>and</b> staff <b>love</b> !                                                                                                                                                                                                         |
| 3 ( $X^3$ ) | <b>this</b> is <b>the</b> new <b>modern</b> breakfast joint <b>to</b> be <b>found</b> around <b>the</b> area . great <b>atmosphere</b> , <b>central</b> location <b>and</b> excellent food . nice variety <b>of</b> selections . great <b>selection</b> of <b>local</b> craft <b>beers</b> , <b>good</b> drinks . quite <b>cheap</b> unless <b>you</b> ask <b>for</b> greater <b>price</b> . <b>very</b> friendly <b>patio</b> and <b>fun</b> staff . love <b>it</b> ! |

Table 8: Example of the progressive generation process with multiple stages from the POINTER model. New additions at each stage are marked as **blue**.

|                         |                                                                                                                                                                                                                                                                                                                                                                        |
|-------------------------|------------------------------------------------------------------------------------------------------------------------------------------------------------------------------------------------------------------------------------------------------------------------------------------------------------------------------------------------------------------------|
| Keywords                | service perfect delicious service awesome good place                                                                                                                                                                                                                                                                                                                   |
| ORACLE                  | yummy excellent <b>service</b> . ordered the carne asada medium rare . it was <b>perfect</b> . and <b>delicious</b> . their customer <b>service</b> was <b>awesome</b> . they were so friendly and made sure all was <b>good</b> . i definitely recommend this <b>place</b> .                                                                                          |
| CGMH                    | great <b>service perfect</b> food and <b>delicious service</b> . <b>awesome</b> place and <b>good place</b> !.                                                                                                                                                                                                                                                         |
| NMSTG                   | <b>service</b> was <b>perfect</b> , <b>delicious</b> and great <b>service awesome</b> service <b>good</b> food . this <b>place</b> will go back .                                                                                                                                                                                                                      |
| POINTER (Greedy, base)  | excellent food , great <b>service</b> , really nice atmosphere , <b>perfect</b> amount of spring rolls , <b>delicious</b> especially the chicken and eel . the <b>service</b> was very friendly and the prices are <b>awesome</b> too . for a female who loves <b>good</b> japanese restaurant , this is definitely your <b>place</b> !                                |
| POINTER (ILBS, base)    | from the food to <b>service</b> . the foods are <b>perfect</b> , they were <b>delicious</b> . and <b>service</b> is beyond expectation . christina was <b>awesome</b> , so many <b>good</b> things about this <b>place</b> .                                                                                                                                           |
| POINTER (Greedy, Large) | absolutely loved the food and very friendly <b>service</b> . i had the chicken , it was cooked <b>perfect</b> and the seafood pasta was thick and <b>delicious</b> and not too heavy though . our <b>service</b> guy at the front bar was so <b>awesome</b> , he made sure we had a <b>good</b> time . would definitely recommend to try this <b>place</b> to anyone ! |
| Wiki zero-shot          | he said the <b>service</b> was <b>perfect</b> , and <b>delicious</b> , and the <b>service</b> that is <b>awesome</b> , and very <b>good</b> in its <b>place</b> .                                                                                                                                                                                                      |

|                         |                                                                                                                                                                                                                                                                                                                                 |
|-------------------------|---------------------------------------------------------------------------------------------------------------------------------------------------------------------------------------------------------------------------------------------------------------------------------------------------------------------------------|
| Keywords                | good drinks love clients tighter great service                                                                                                                                                                                                                                                                                  |
| ORACLE                  | <b>great</b> atmosphere , good food and <b>drinks</b> . i <b>love</b> coming here in the fall to spring to meet with <b>clients</b> . their inside is a little small and makes summer a bit <b>tighter</b> , but still a <b>great</b> staff with excellent <b>service</b> .                                                     |
| CGMH                    | <b>good drinks</b> . i <b>love</b> how out <b>clients</b> are <b>tighter</b> . <b>great</b> customer <b>service</b> .                                                                                                                                                                                                           |
| NMSTG                   | such <b>good</b> place with i love the mushroom <b>drinks</b> . the menu they <b>love</b> the <b>clients</b> . and <b>tighter</b> out the menu are <b>great service</b> .                                                                                                                                                       |
| POINTER (Greedy, base)  | this place is <b>good</b> . they have a wide variety of <b>drinks</b> . this really fits your taste . <b>love</b> the cozy bar that allows <b>clients</b> to be able to fit very tightly and <b>tighter</b> , better blending with the crowd . <b>great</b> coffee , reasonable prices , and friendly <b>service</b> !          |
| POINTER (ILBS, base)    | nice place , with <b>good</b> vibe . nice mix of <b>drinks</b> and intimate space . what i really <b>love</b> about was there were so more mature <b>clients</b> , and they can fit in a <b>tighter</b> timeline . overall , <b>great</b> atmosphere and excellent <b>service</b> .                                             |
| POINTER (Greedy, Large) | really like this place . has a <b>good</b> dj , good atmosphere and cool <b>drinks</b> and quite nice lounge area . i <b>love</b> this idea of having fun on your <b>clients</b> and rubbing your feet to stand up <b>tighter</b> than other ones . <b>great</b> variety of drinks and pretty quick <b>service</b> at the bar ! |
| Wiki zero-shot          | she is a <b>good</b> at <b>drinks</b> , and in <b>love</b> for him and all his <b>clients</b> , and he enjoys a <b>tighter</b> schedule and has a <b>great</b> food and a generous <b>service</b> .                                                                                                                             |



|                         |                                                                                                                                                                                                                                                                                                                                                               |
|-------------------------|---------------------------------------------------------------------------------------------------------------------------------------------------------------------------------------------------------------------------------------------------------------------------------------------------------------------------------------------------------------|
| Keywords                | joint great food great drinks greater staff                                                                                                                                                                                                                                                                                                                   |
| ORACLE                  | apteka is seriously all around the best vegan <b>joint</b> in the burgh . <b>great food</b> , <b>great drinks</b> , <b>greater staff</b> .                                                                                                                                                                                                                    |
| CGMH                    | very cool <b>joint</b> with <b>great food</b> , <b>great drinks</b> and even <b>greater staff</b> . !                                                                                                                                                                                                                                                         |
| NMSTG                   | awesome <b>joint</b> . <b>great</b> service . <b>great food</b> great <b>drinks</b> . good to <b>greater</b> and great <b>staff</b> !                                                                                                                                                                                                                         |
| POINTER (Greedy, base)  | my favorite local <b>joint</b> around old town . <b>great</b> atmosphere , amazing <b>food</b> , delicious and delicious coffee , <b>great</b> wine selection and delicious cold <b>drinks</b> , oh and maybe even a <b>greater</b> patio space and energetic front desk <b>staff</b> .                                                                       |
| POINTER (ILBS, base)    | the best breakfast <b>joint</b> in charlotte . <b>great</b> service and amazing <b>food</b> . they have <b>great</b> selection of <b>drinks</b> that suits the <b>greater</b> aesthetic of the <b>staff</b> .                                                                                                                                                 |
| POINTER (Greedy, Large) | this is the new modern breakfast <b>joint</b> to be found around the area . <b>great</b> atmosphere , central location and excellent <b>food</b> . nice variety of selections . <b>great</b> selection of local craft beers , good <b>drinks</b> . quite cheap unless you ask for <b>greater</b> price . very friendly patio and fun <b>staff</b> . love it ! |
| Wiki zero-shot          | it is a joint owner of the <b>great</b> society of irish <b>food</b> , and the <b>great</b> britain and soft <b>drinks</b> , and the <b>greater</b> britain and its <b>staff</b> .                                                                                                                                                                            |

|                         |                                                                                                                                                                                                                                                                                                                                                         |
|-------------------------|---------------------------------------------------------------------------------------------------------------------------------------------------------------------------------------------------------------------------------------------------------------------------------------------------------------------------------------------------------|
| Keywords                | service polite professional affordable work safe tree                                                                                                                                                                                                                                                                                                   |
| ORACLE                  | aron's tree <b>service</b> were very <b>polite</b> and <b>professional</b> . they are very <b>affordable</b> . they arrived a little early and got right to <b>work</b> . they were quick and <b>safe</b> . they cleaned up and hauled out the <b>tree</b> trimmings . i highly recommend them .                                                        |
| CGMH                    | excellent customer <b>service</b> , <b>polite</b> , <b>professional</b> , and <b>affordable work</b> , <b>safe</b> bike <b>tree</b> .                                                                                                                                                                                                                   |
| NMSTG                   | excellent food and <b>service</b> and are amazing service and <b>polite</b> and <b>professional</b> . <b>affordable</b> it <b>work</b> out <b>safe</b> on sun <b>tree</b> !                                                                                                                                                                             |
| POINTER (Greedy, base)  | amazing customer <b>service</b> . so <b>polite</b> , and very <b>professional</b> , and very <b>affordable</b> . such great <b>work</b> done at the <b>safe</b> end of a <b>tree</b> .                                                                                                                                                                  |
| POINTER (ILBS, base)    | excellent customer <b>service</b> , very <b>polite</b> , and very <b>professional</b> . honest and <b>affordable</b> pricing . i will definitely get the <b>work</b> done here for the <b>safe</b> parts of my <b>tree</b> .                                                                                                                            |
| POINTER (Greedy, Large) | diane provides customers with great customer <b>service</b> . technician mike was very <b>polite</b> and helpful . clean facility , very <b>professional</b> , and always responsive . quick and <b>affordable</b> as well . i had very nice <b>work</b> done . we have now found someone <b>safe</b> . thank you big two buck <b>tree</b> shrub care ! |
| Wiki zero-shot          | customer <b>service</b> should be more <b>polite</b> , and more <b>professional</b> , and more <b>affordable</b> , and will <b>work</b> in a <b>safe</b> place under the family <b>tree</b> .                                                                                                                                                           |

|                         |                                                                                                                                                                                                                                                                                                                                                                                                          |
|-------------------------|----------------------------------------------------------------------------------------------------------------------------------------------------------------------------------------------------------------------------------------------------------------------------------------------------------------------------------------------------------------------------------------------------------|
| Keywords                | hesitate give customers chicken rice<br>decent list                                                                                                                                                                                                                                                                                                                                                      |
| ORACLE                  | i <b>hesitate</b> to <b>give</b> them the five stars they deserve because they have a really small dining area and more <b>customers</b> , selfishly , would complicate things for me . <b>chicken</b> panang is quite good with a superb brown <b>rice</b> . <b>decent</b> wine <b>list</b> . after three visits the wait staff remembered what i like ( complicated ) and always get the order right . |
| CGMH                    | they <b>hesitate</b> to <b>give customers</b> their <b>chicken</b> fried <b>rice</b> and a <b>decent</b> wine <b>list</b> .                                                                                                                                                                                                                                                                              |
| NMSTG                   | they <b>hesitate</b> to an wonderful time to <b>give</b> it about a table , love the <b>customers chicken rice</b> and dishes seafood and <b>decent</b> at the <b>list</b> .                                                                                                                                                                                                                             |
| POINTER (Greedy, base)  | i just did not even <b>hesitate</b> to admit , i should <b>give</b> credit cards to my <b>customers</b> here . the beijing <b>chicken</b> and fried <b>rice</b> were spot on , a <b>decent</b> side on my favorite <b>list</b> .                                                                                                                                                                         |
| POINTER (ILBS, base)    | i don't have to <b>hesitate</b> that they should <b>give</b> five stars . i will be one of their repeat <b>customers</b> . like the basil <b>chicken</b> and basil fried <b>rice</b> , it was <b>decent</b> on my <b>list</b> .                                                                                                                                                                          |
| POINTER (Greedy, Large) | service is very slow , don ' t <b>hesitate</b> to tell manager to <b>give</b> some feed-backs as their job is to take care of their <b>customers</b> . had the vegetable medley soup and <b>chicken</b> . both were cooked well . the garlic <b>rice</b> did not have the vegetable and was fairly <b>decent</b> . they are changing the flavor and <b>list</b> of menu items .                          |
| Wiki zero-shot          | he did not <b>hesitate</b> himself to <b>give</b> it to his <b>customers</b> , such as <b>chicken</b> , and steamed <b>rice</b> , a very <b>decent</b> item on the <b>list</b> .                                                                                                                                                                                                                         |

|                         |                                                                                                                                                                                                                                                                                                                                                        |
|-------------------------|--------------------------------------------------------------------------------------------------------------------------------------------------------------------------------------------------------------------------------------------------------------------------------------------------------------------------------------------------------|
| Keywords                | good potential bad maintained replaced dirty disgusting                                                                                                                                                                                                                                                                                                |
| ORACLE                  | has <b>good potential</b> but very <b>bad maintained</b> . the padding is done , needs to be <b>replaced</b> , holes everywhere . so are those huge flowers or what ever those are . ripped . very <b>dirty</b> too . there was a a very dirty towel laying on the floor <b>disgusting</b> . please the city of vegas come and clean it !              |
| CGMH                    | <b>good potential</b> but <b>bad</b> service. not <b>maintained</b> . it <b>replaced</b> a <b>dirty</b> box . <b>disgusting</b> .                                                                                                                                                                                                                      |
| NMSTG                   | do a <b>good</b> price . not like the and <b>potential bad maintained</b> has disgusting . <b>replaced</b> been , <b>dirty</b> and <b>disgusting</b> .                                                                                                                                                                                                 |
| POINTER (Greedy, base)  | the food was very <b>good</b> . it really has more <b>potential</b> maybe , but it smells really <b>bad</b> . its not very well <b>maintained</b> either . trash cans were <b>replaced</b> only when they were <b>dirty</b> . the floors were utterly <b>disgusting</b> .                                                                              |
| POINTER (ILBS, base)    | the food is really <b>good</b> . this location has <b>potential</b> to be pretty <b>bad</b> and not very well <b>maintained</b> when it was <b>replaced</b> , its super <b>dirty</b> , just plain <b>disgusting</b> .                                                                                                                                  |
| POINTER (Greedy, Large) | this gym is not so <b>good</b> . overall it has a lot of <b>potential</b> for being better but it is too <b>bad</b> that it is not clean and un <b>maintained</b> and towels are in desperate need to be <b>replaced</b> regularly . the floors are very <b>dirty</b> and the higher floors have become filthy <b>disgusting</b> when i visited here . |
| Wiki zero-shot          | it is <b>good</b> it has no <b>potential</b> , and the <b>bad</b> taste can be <b>maintained</b> until they are <b>replaced</b> by a <b>dirty</b> , and <b>disgusting</b> one .                                                                                                                                                                        |

|                         |                                                                                                                                                                                                                                                                                                                        |
|-------------------------|------------------------------------------------------------------------------------------------------------------------------------------------------------------------------------------------------------------------------------------------------------------------------------------------------------------------|
| Keywords                | love animal style long line expected quick                                                                                                                                                                                                                                                                             |
| ORACLE                  | who doesn't <b>love</b> in and out . <b>animal</b> style is a must . <b>long line</b> but <b>expected</b> , it goes <b>quick</b> anyways so don't let that discourage you .                                                                                                                                            |
| CGMH                    | <b>love</b> this place . <b>animal style</b> food . <b>long line</b> than <b>expected</b> for <b>quick</b> .                                                                                                                                                                                                           |
| NMSTG                   | <b>love animal</b> chicken . it was <b>style long</b> a bit so good . the <b>line</b> is it was even on on a time and we <b>expected</b> to go but <b>quick</b> .                                                                                                                                                      |
| POINTER (Greedy, base)  | great little breakfast spot . i <b>love</b> having the double with <b>animal style</b> fries and protein style etc . have a super <b>long</b> wait <b>line</b> , but its just as <b>expected</b> and it always moves pretty <b>quick</b> too .                                                                         |
| POINTER (ILBS, base)    | y all you just gotta <b>love</b> about this place is the double <b>animal style</b> and protein style . it was a <b>long line</b> , but i <b>expected</b> it to be <b>quick</b> .                                                                                                                                      |
| POINTER (Greedy, Large) | great burger and good price . i <b>love</b> that they have non chain locations . i like the <b>animal style</b> fries too . have to wait <b>long</b> as there is always traffic but the <b>line</b> can be much shorter than i had <b>expected</b> and they are always send out pretty <b>quick</b> . very impressed ! |
| Wiki zero-shot          | he also has <b>love</b> with the <b>animal</b> and his <b>style</b> , and was <b>long</b> as the finish <b>line</b> , and was <b>expected</b> to be <b>quick</b> .                                                                                                                                                     |

|                         |                                                                                                                                                                                                                                                                                                                       |
|-------------------------|-----------------------------------------------------------------------------------------------------------------------------------------------------------------------------------------------------------------------------------------------------------------------------------------------------------------------|
| Keywords                | great great service happy found close home                                                                                                                                                                                                                                                                            |
| ORACLE                  | <b>great</b> sushi and <b>great service</b> . i m really <b>happy</b> to have <b>found</b> a good sushi place so <b>close</b> to <b>home</b> !                                                                                                                                                                        |
| CGMH                    | <b>great</b> price and <b>great</b> customer <b>service</b> . very <b>happy</b> that i <b>found</b> this place <b>close</b> to my <b>home</b> .                                                                                                                                                                       |
| NMSTG                   | <b>great</b> food and <b>great service</b> . a <b>happy</b> and <b>found</b> a year in <b>close</b> for them . keep them <b>home</b> here .                                                                                                                                                                           |
| POINTER (Greedy, base)  | amazing food . <b>great</b> quality food . <b>great</b> prices and friendly <b>service</b> staff . so <b>happy</b> and surprised to have finally <b>found</b> such a wonderful nail salon so <b>close</b> to my work and <b>home</b> .                                                                                |
| POINTER (ILBS, base)    | this is just <b>great</b> food . <b>great</b> food and wonderful <b>service</b> . very <b>happy</b> to have finally <b>found</b> a chinese restaurant <b>close</b> to my <b>home</b> .                                                                                                                                |
| POINTER (Greedy, Large) | wow . i have been here twice . <b>great</b> times here . food always has been <b>great</b> and the customer <b>service</b> was wonderful . i am very <b>happy</b> that we finally <b>found</b> our regular pad thai restaurant that is <b>close</b> to where we work now and our <b>home</b> . pleasantly surprised ! |
| Wiki zero-shot          | he was a <b>great</b> teacher and a <b>great</b> love of the <b>service</b> he was very <b>happy</b> , and he <b>found</b> himself in the <b>close</b> to his <b>home</b> .                                                                                                                                           |

## D Additional Human Evaluation Results

We present the additional human evaluation results on POINTER large model vs base model in table 11. In general, for the news dataset the results are mixed. For the yelp dataset, the large model wins with a large margin. All results are still far away from the human oracle in all three aspects.

## E Additional Automatic Evaluation Results

We provide the full evaluation result data including Wikipedia zero-shot learning results in Table 9



| Method           | NIST        |             | BLEU          |              | METEOR        | Entropy<br>E-4 | Dist   |        | PPL         | Avg Len |
|------------------|-------------|-------------|---------------|--------------|---------------|----------------|--------|--------|-------------|---------|
|                  | N-2         | N-4         | B-2           | B-4          |               |                | D-1    | D-2    |             |         |
| Greedy (+Wiki)   | 3.04        | 3.06        | 13.01%        | 2.51%        | <b>16.38%</b> | 10.22          | 11.10% | 57.78% | <b>56.7</b> | 31.32   |
| ILBS (+Wiki)     | 3.20        | 3.22        | 14.00%        | 2.99%        | 15.71%        | 9.86           | 13.17% | 61.22% | 66.4        | 22.59   |
| Greedy (+Wiki,L) | <b>3.28</b> | <b>3.30</b> | <b>14.04%</b> | <b>3.04%</b> | 15.90%        | 10.09          | 12.23% | 60.86% | <b>54.7</b> | 27.99   |
| Wiki zero-shot   | 2.80        | 2.82        | 11.38%        | 1.84%        | 15.12%        | 9.73           | 14.33% | 53.97% | 62.9        | 20.68   |
| Human            | -           | -           | -             | -            | -             | 10.05          | 11.80% | 62.44% | 47.4        | 27.85   |

Table 9: Additional evaluation results on the News dataset. ILBS denotes beam search. “+Wiki” denotes fine-tuning on the Wiki-pretrained model. “Human” represents the held-out human reference. “Wiki zero-shot” represents zero-shot generation from the pre-trained model.

| Method         | NIST        |             | BLEU          |              | METEOR | Entropy<br>E-4 | Dist   |        | PPL         | Avg Len |
|----------------|-------------|-------------|---------------|--------------|--------|----------------|--------|--------|-------------|---------|
|                | N-2         | N-4         | B-2           | B-4          |        |                | D-1    | D-2    |             |         |
| Greedy (+Wiki) | 3.27        | 3.30        | 15.63%        | 3.32%        | 16.14% | 10.64          | 7.51%  | 46.12% | 71.9        | 48.22   |
| ILBS (+Wiki)   | 3.34        | 3.38        | 16.68%        | 3.65%        | 15.57% | 10.44          | 9.43%  | 50.66% | 61.0        | 35.18   |
| Large (+Wiki)  | <b>3.49</b> | <b>3.53</b> | <b>16.78%</b> | <b>3.79%</b> | 16.69% | 10.56          | 6.94%  | 41.2%  | <b>55.5</b> | 48.05   |
| Wiki zero-shot | 0.86        | 0.87        | 8.56%         | 1.30%        | 12.85% | 9.90           | 10.09% | 41.97% | 62.9        | 26.80   |
| Human          | -           | -           | -             | -            | -      | 10.70          | 10.67% | 52.57% | 55.4        | 50.36   |

Table 10: Additional evaluation results on the Yelp dataset. ILBS denotes beam search. “+Wiki” denotes fine-tuning on the Wiki-pretrained model. “Human” represents the held-out human reference. “Wiki zero-shot” represents zero-shot generation from the pre-trained model.

| Informativeness: A and B, which is more semantically meaningful and consistent? |              |       |               |               |                |              |        |              |                   |
|---------------------------------------------------------------------------------|--------------|-------|---------------|---------------|----------------|--------------|--------|--------------|-------------------|
| News dataset                                                                    |              |       |               |               | Yelp dataset   |              |        |              |                   |
| System A                                                                        | Neutral      |       | System B      |               | System A       | Neutral      |        | System B     |                   |
| POINTER(large)                                                                  | 35.4%        | 27.7% | <b>36.9 %</b> | POINTER(base) | POINTER(large) | <b>41.4%</b> | 26.6%  | 32.1 %       | POINTER(base) *** |
| POINTER(large)                                                                  | 20.3%        | 22.7% | <b>57.1%</b>  | Human ***     | POINTER(large) | 27.2%        | 24.4%  | <b>48.5%</b> | Human ***         |
| Fluency: A and B, which is more grammatical and fluent?                         |              |       |               |               |                |              |        |              |                   |
| News dataset                                                                    |              |       |               |               | Yelp dataset   |              |        |              |                   |
| System A                                                                        | Neutral      |       | System B      |               | System A       | Neutral      |        | System B     |                   |
| POINTER(large)                                                                  | <b>38.4%</b> | 28.5% | 33.2 %        | POINTER(base) | POINTER(large) | <b>41.1%</b> | 28.1%  | 30.8 %       | POINTER(base) *** |
| POINTER(large)                                                                  | 16.7%        | 15.8% | <b>67.5%</b>  | Human ***     | POINTER(large) | 27.1%        | 21.9%  | <b>51.1%</b> | Human ***         |
| Informativeness: A and B, which is more informative?                            |              |       |               |               |                |              |        |              |                   |
| News dataset                                                                    |              |       |               |               | Yelp dataset   |              |        |              |                   |
| System A                                                                        | Neutral      |       | System B      |               | System A       | Neutral      |        | System B     |                   |
| POINTER(large)                                                                  | 32.1%        | 27.6% | <b>40.4 %</b> | POINTER(base) | POINTER(large) | <b>41.6%</b> | 25.0 % | 33.4 %       | POINTER(base) *** |
| POINTER(large)                                                                  | 31.9%        | 17.1% | <b>51.0%</b>  | Human ***     | POINTER(large) | 35.9%        | 14.7%  | <b>49.4%</b> | Human ***         |

Table 11: **Human Evaluation** on two datasets for semantic consistency, fluency and informativeness, showing preferences (%) for our POINTER(large) model vis-a-vis POINTER(base) model and real human responses. Numbers in bold indicate the most preferred systems. Significant differences ( $p \leq 0.001$ ) are indicated as \*\*\*.

and Table 10. Note that zero-shot generations from Wikipedia pre-trained model yield the lowest perplexity, presumably because the Wikipedia dataset is large enough so that the model trained on it can learn language variability, thus delivering fluent generated results.

## F Inference Details

During inference time, we use a decaying schedule to discourage the model from generating non-

interesting tokens, including [NOI] and some other special tokens, punctuation and stop words. To do this, we use a decay multiplier  $\eta$  on the logits of these tokens before computing the softmax. The  $\eta$  is set to be  $\eta = \min(0.5 + \lambda * s)$ , where  $s$  is the current stage and  $\lambda$  is an annealing hyper-parameter. In most of the experiments,  $\lambda$  is set at 0.5

## G Human Evaluation Template

See Figure 2 for human evaluation template

Constrained Text Generation

Preview Design + Debug mode

Disable Debug

Time Left: 01:02

User: Chris Brockett

Report a technical issue

Instructions

Compare the two short texts shown below, and answer the questions. The first question should be answered in light of the KEY TERMS shown. In the second and third questions, you should ignore the key terms in making your judgment.

For the purposes of this task, please ignore minor issues in punctuation and capitalization.

**TEXT #1:** this place is no joke. there is to order to replace the review. their hearing a manager to contacted and I back one was the competitor down.

**TEXT #2:** if I could give this place zero stars and give them an order. kind of disappointed. I was hearing some bad comments from a manager who heard of this complaint, and contacted me and offered to get my business back. I find a direct competitor in the market again.

**KEY TERMS:** place order hearing manager contacted back competitor

Semantics:

Which of the two texts is more semantically meaningful and consistent in light of the key terms?

☐ Clearly Text #1  
☐ Maybe Text #1  
☐ Neither  
☐ Maybe Text #2  
☐ Clearly Text #2

Informativeness:

IGNORING the key terms, which of the two texts is more informative (has more specific content)?

☐ Clearly Text #1  
☐ Maybe Text #1  
☐ Neither  
☐ Maybe Text #2  
☐ Clearly Text #2

Grammar and Fluency:

Which of the two texts is more grammatical and fluent?

☐ Clearly Text #1  
☐ Maybe Text #1  
☐ Neither  
☐ Maybe Text #2  
☐ Clearly Text #2

Submit

Figure 2: Human evaluation template.
